# Supplementary material for: Reducing Commutativity Verification to Reachability with Differencing Abstractions
Source: arXiv:2004.08450 source file (2020-04-17)
Supplement: Supplementary file 1 [file appendix.tex]

%\section{Omitted Proofs}
%\label{apx:proofs}
%\ifextended\else
%\subsection{Proof sketch of Theorem \ref{thm:abstraction}.}
%\begin{proof}[sketch of Theorem \ref{thm:abstraction}]
%	\input{proof1}
%\end{proof}
%\fi
%\subsection{Proof sketch of Theorem \ref{thm:soundness}.}
%\begin{proof}[sketch of Theorem \ref{thm:soundness}]
%	\input{proof2}
%\end{proof}
%
